# Supplementary material for: A novel mathematical model of heterogeneous cell proliferation
Source: arXiv:2003.03024 source file (2020-07-24)
Supplement: Supplementary file 1 [file FastSlow_SupplementaryMaterial_arXiv.tex]

\documentclass[11pt]{article}
\usepackage{amsmath, afterpage, pdflscape, changepage, multirow, multicol, cleveref, hhline, array, xcolor, verbatim, graphicx, url, fancyhdr, etoolbox, bigstrut, cite, setspace, float, xr, amssymb, mathtools, capt-of, amsthm}
\usepackage[font=small,labelfont=bf]{caption}
\usepackage[hang]{footmisc}
\usepackage[USenglish]{babel}
\usepackage[USenglish]{isodate}
\usepackage[hmargin=2cm,top=1.5cm,bottom=1.5cm]{geometry}
\usepackage[inline]{enumitem}

\doublespacing

\AtBeginEnvironment{tabular}{\onehalfspacing}

\setlength{\emergencystretch}{5pt}

\Crefname{equation}{Eq}{Eqs}

\newcommand{\RR}{\mathbb{R}}
\newcommand*\mean[1]{\overline{#1}}

\let\svthefootnote\thefootnote
\newcommand\blankfootnote[1]{%
  \let\thefootnote\relax\footnotetext{#1}%
  \let\thefootnote\svthefootnote%
}

\theoremstyle{remark}

\title{\LARGE A novel mathematical model of heterogeneous cell proliferation}

\author{\normalsize S. T. Vittadello, S. W. McCue, G. Gunasingh, N. K. Haass, M. J. Simpson}

\fancypagestyle{specialfooter}{%
\fancyhf{}

%\vspace{0.7in}
\fancyfoot[R]{\footnotesize \emph{\today}}
}

\pagestyle{plain}

%\externaldocument[main-]{FastSlow_Revision_arXiv}
% These labels are from FastSlow_Revision_arXiv.aux, modified with 'main-',
% as referencing an external document doesn't work in arXiv.
\newlabel{main-thrm:NonNeg}{{2}{10}}
\newlabel{main-P(t)}{{3}{10}}
\newlabel{main-eq:FS1}{{2}{8}}
\newlabel{main-eq:FS2}{{3}{8}}
\newlabel{main-fig:Fig1}{{1}{3}}
\newlabel{main-thrm:Exist}{{4}{12}}
\newlabel{main-eq:f}{{14}{11}}
\newlabel{main-prop:Equil0}{{6}{15}}
\newlabel{main-eq:Sum}{{12}{9}}
\newlabel{main-eq:Transcendental}{{25}{16}}
\newlabel{main-eq:history1}{{9}{9}}
\newlabel{main-eq:history2}{{10}{9}}

\begin{document}
\captionsetup[figure]{name={Figure}}
%Begin title page
\makeatletter
\begin{titlepage}
\thispagestyle{specialfooter}
{\Large Supplementary Material for: \hfill} \\[2cm]
\centering
\@title\\
\vspace{5mm}
\@author\\
\vspace{5mm}
\cleanlookdateon
%\@date\\
\vspace{0mm}
\end{titlepage}
\makeatother

%End title page

\tableofcontents

\newpage

\section{Experimental}
We briefly describe the materials and methods employed to obtain our experimental data for the durations of cells in G1 and S/G2/M phases, shown in Figure~\ref{fig:FigS1}.
\begin{figure}
\includegraphics[width=0.9\textwidth]{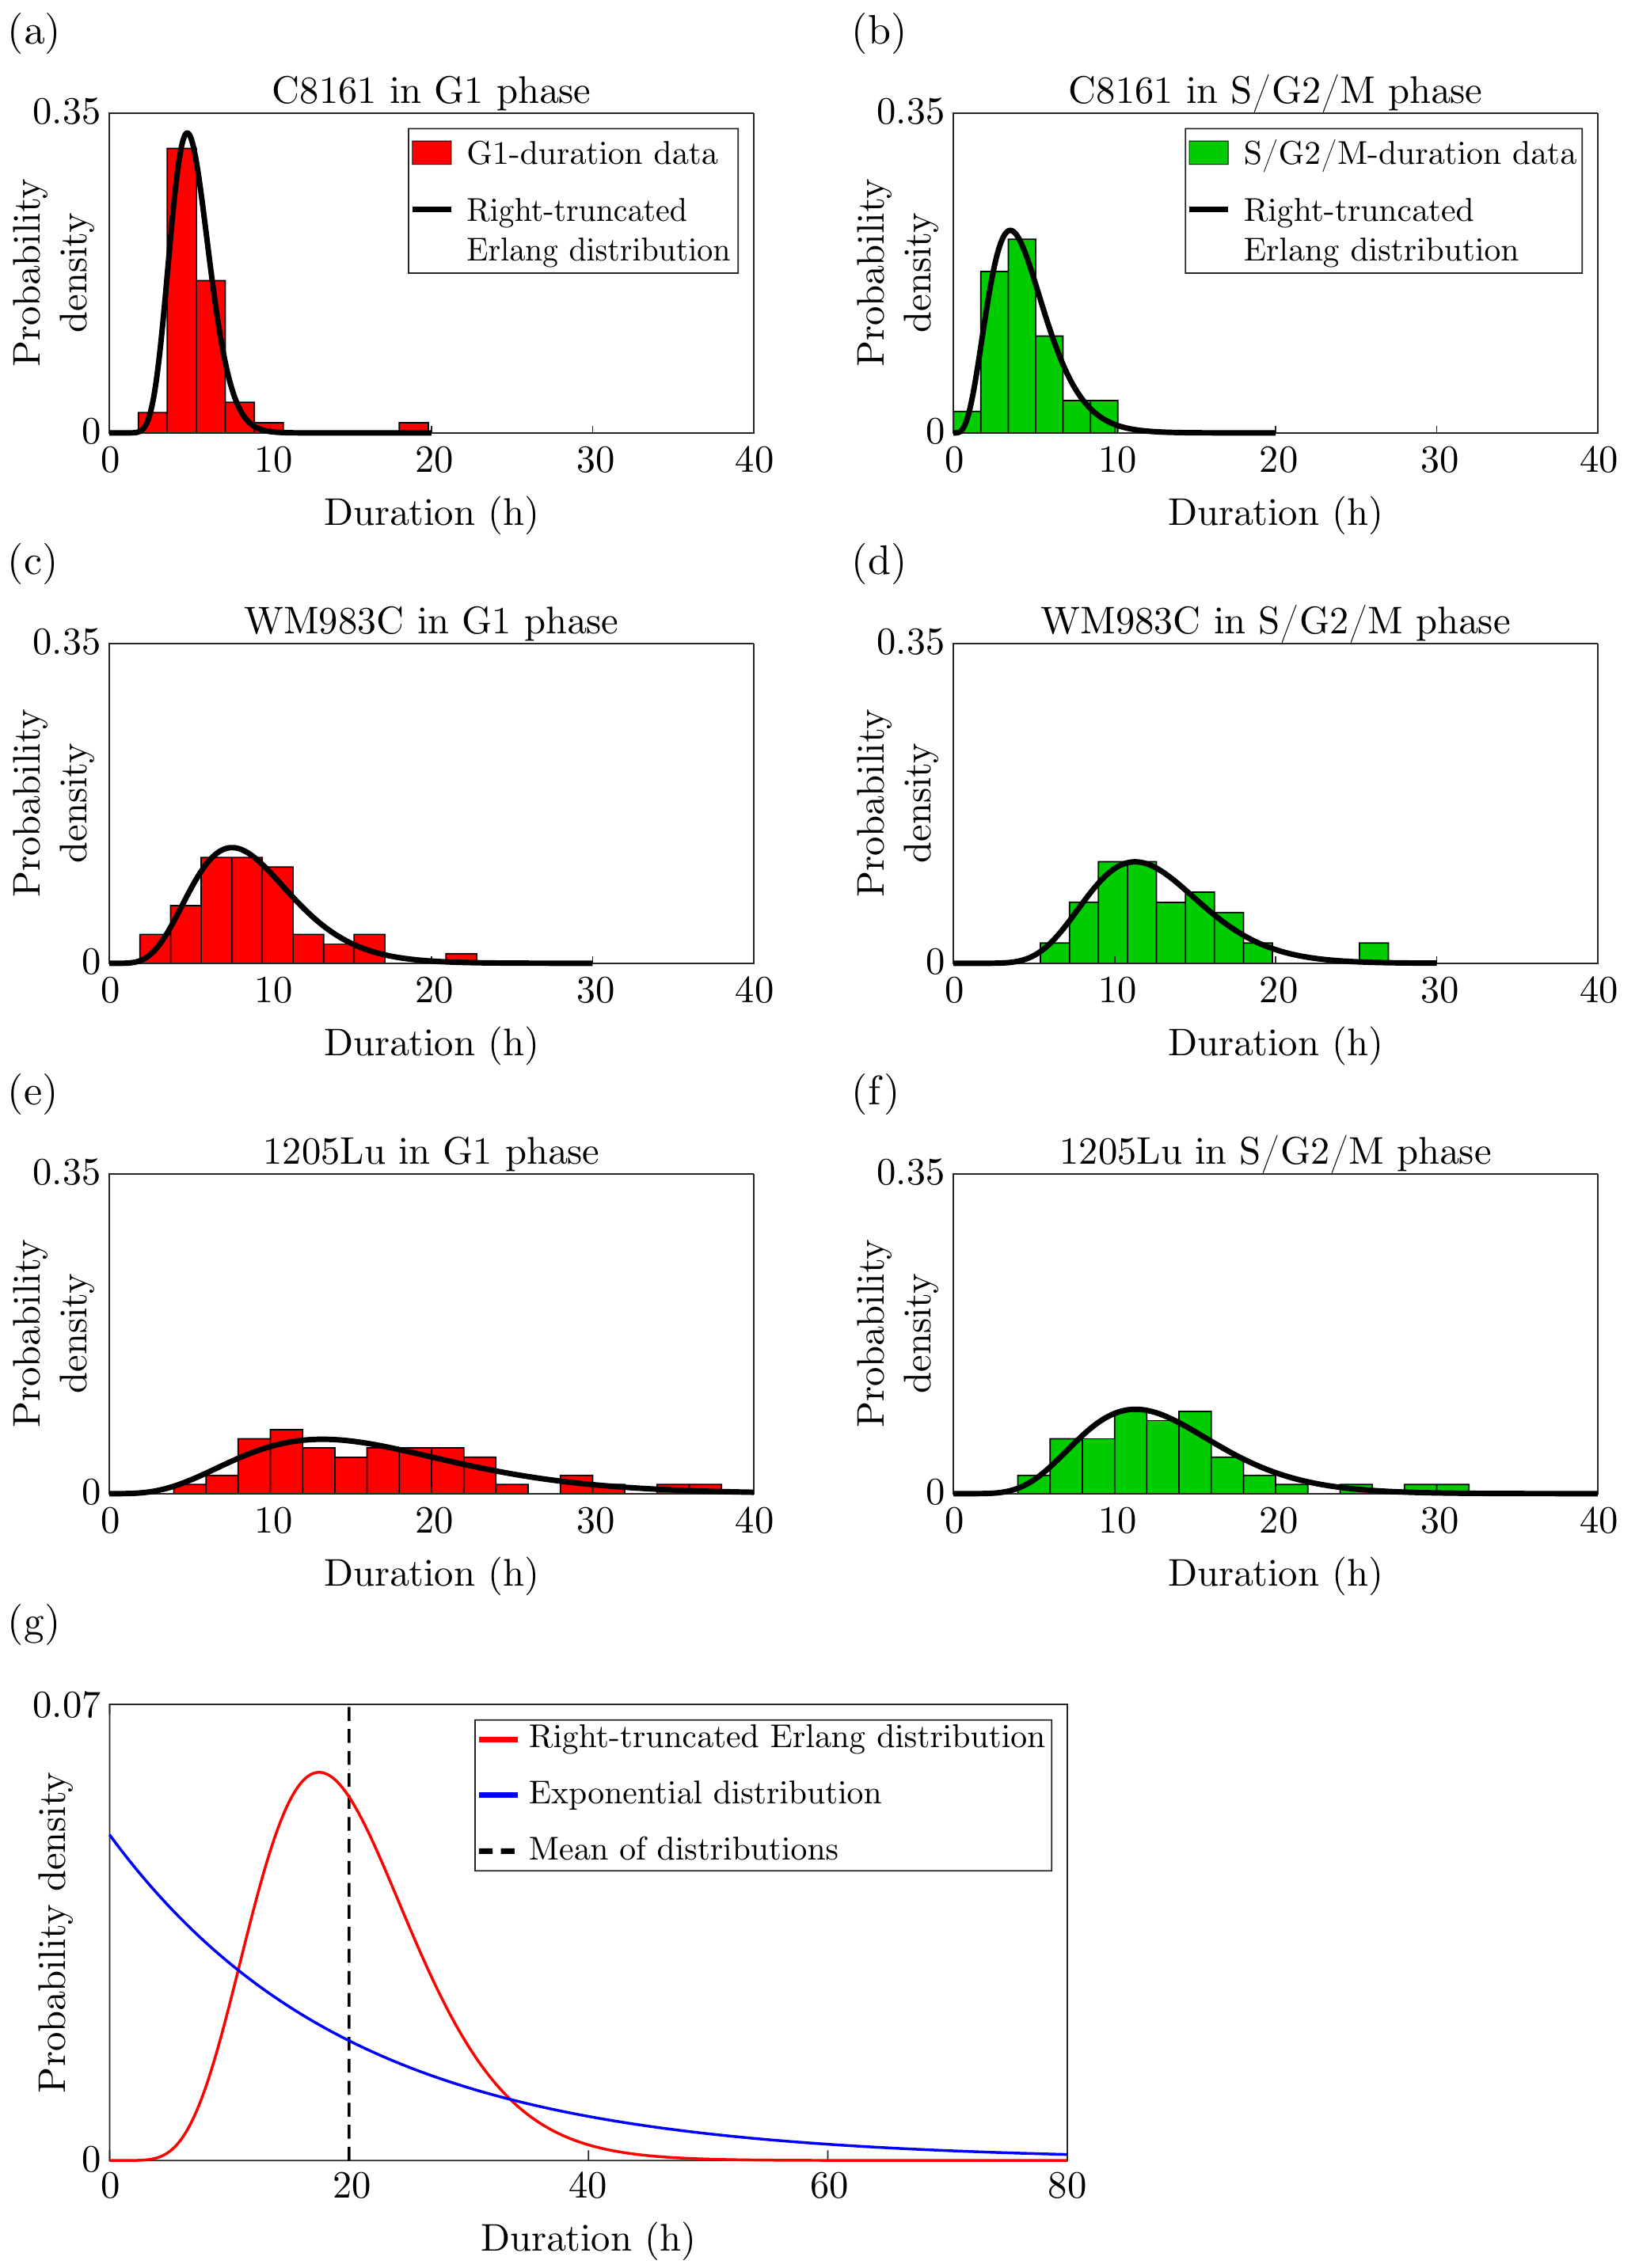}
\caption{Histograms of G1- and S/G2/M-phase duration data with best fits of the right-truncated Erlang distribution in Equation~\eqref{eq:TruncErlang}, and a comparison of the probability density functions of the right-truncated Erlang and exponential distributions. Each histogram corresponds to 50 cells. The best-fit parameters for the right-truncated Erlang distribution are: (a) $\text{RTE}(17,3.3 \, \text{h}^{-1},20 \, \text{h})$; (b) $\text{RTE}(5,1.1 \, \text{h}^{-1},20 \, \text{h})$; (c) $\text{RTE}(7,0.79 \, \text{h}^{-1},30 \, \text{h})$; (d) $\text{RTE}(11,0.89 \, \text{h}^{-1},30 \, \text{h})$; (e) $\text{RTE}(5,0.30 \, \text{h}^{-1},40 \, \text{h})$; (f) $\text{RTE}(8,0.62 \, \text{h}^{-1},40 \, \text{h})$. (g) Probability density functions of the right-truncated Erlang and exponential distributions, for $\text{RTE}(8,0.4 \, \text{h}^{-1},80 \, \text{h})$ and $\text{Exp}(0.05 \, \text{h}^{-1})$. The exponential distribution has mean 20 h, and the right-truncated Erlang distribution has mean 20.0000 h (to four decimal places)}
\label{fig:FigS1}
\end{figure}
Further experimental details are given in \cite{Vittadello2020}. Each histogram is constructed using data from 50 individual cells.

Our experimental data consist of microscopy time-series images of two-dimensional cell proliferation assays using the three human melanoma cell lines C8161 (kindly provided by Mary Hendrix, Chicago, IL, USA), WM983C and 1205Lu (both kindly provided by Meenhard Herlyn, Philadelphia, PA, USA), which have cell cycle durations of approximately 21, 23 and 37 h, respectively \cite{Haass2014}. The cell lines were genotypically characterised \cite{Davies2009,Hoek2006,Smalley2007,Smalley2007a}, grown as described in \cite{Spoerri2017}, and authenticated by STR fingerprinting (QIMR Berghofer Medical Research Institute, Herston, Australia).

We maintain the cell cultures to prevent any induced synchronisation from cell cycle arrest in G1 phase, by passaging the cells every three days, and on the day prior to setting up an experiment, to maintain a subconfluent cell density and a fresh growth medium.

Experimental investigation of the progression of the cell cycle is visually enabled with fluorescent ubiquitination-based cell cycle indicator (FUCCI) technology \cite{Sakaue_Sawano2008}. FUCCI consists of two genetically-encoded reporters that enable visualisation of the cell cycle of individual live cells: when the cell is in G1 phase the nucleus fluoresces red, and when the cell is in S/G2/M phase the nucleus fluoresces green (Figure~\ref{main-fig:Fig1} in the main document). During the transition from G1 to S phase, called early S, both reporters fluoresce and the nucleus appears yellow. FUCCI is utilised in experimental studies of the cycling dynamics of cells in tumours \cite{Haass2014}, and reveals the differential cycling of the cell population.

\clearpage

\section{Experimental data and models for cell cycle durations}
Standard deterministic mathematical models of cell proliferation, such as exponential~\eqref{eq:EXPmodel} and logistic~\eqref{eq:LOGmodel} growth models,
\begin{align}
\frac{\mathrm{d}P(t)}{\mathrm{d}t} &= r P(t) \label{eq:EXPmodel},\\[0.5cm]
\frac{\mathrm{d}P(t)}{\mathrm{d}t} &= r P(t) \bigg(1 - \frac{P(t)}{K}\bigg), \label{eq:LOGmodel}
\end{align}
where $P(t)$ is the population density at time $t$, $r$ is the intrinsic growth rate, and $K$ is the carrying capacity density, are based on cell cycle durations with an exponential distribution $\text{Exp}(\theta)$ for rate $\theta$. Realising Equations~\eqref{eq:EXPmodel} and \eqref{eq:LOGmodel} as stochastic pure birth processes yields continuous-time homogeneous Markov chains with exponentially-distributed durations of cell cycle residence \cite{Allen2010}. Experimental investigations, however, suggest that the duration of the cell cycle, and in particular each cell cycle phase, is not exponentially distributed \cite{Weber2014,Yates2017,Vittadello2019,Chao2019,Gavagnin2019}. Rather, it is often found that the hypoexponential distribution, characterised as the sum of $k$ independent exponential random variables with distinct rate parameters $\lambda_i$, for $i = 1$, $\ldots, k$, is a reasonable distribution for cell cycle duration \cite{Weber2014,Yates2017,Vittadello2019,Chao2019,Gavagnin2019}. The hypoexponential distribution generalises the Erlang distribution for which the exponential random variables have the same rate parameter $\lambda$. Since the exponential distribution allows for a relatively large probability of arbitrarily small cell cycle durations, ordinary differential equations such as \eqref{eq:EXPmodel} and \eqref{eq:LOGmodel} tend to overestimate the population growth rate, particularly for slow-proliferating cells.

We consider only bounded distributions for their greater biological realism. A particular example of a bounded delay kernel that may be relevant when modelling the cell cycle is the probability density for the right-truncated Erlang distribution. The probability density for the Erlang distribution is
\begin{equation}\label{eq:Erlang}
g(z) = \frac{\lambda^k z^{k-1} e^{-\lambda z}}{(k-1)!}\, ,\ \text{for} \ z \in [0,\infty),
\end{equation}
where $k$ is the shape parameter, $\lambda$ is the rate parameter, and the mean is $k / \lambda$. Restricting the Erlang distribution to the bounded interval $[0,U]$, where $U \in (0,\infty)$, gives the right-truncated Erlang distribution which has probability density
\begin{equation}\label{eq:TruncErlang}
g_{\ast}(z) = \frac{g(z)}{\displaystyle \int_{0}^{U} g(w)\, \mathrm{d}w}\, ,\ \text{for} \ z \in [0,U].
\end{equation}
We also show in Figure~\ref{fig:FigS1} the best fit to the data for the right-truncated Erlang distribution $\text{RTE}(k,\lambda,U)$, where the shape $k$ and rate $\lambda$ correspond to the Erlang distribution, and $U$ is the right-truncation point of the Erlang distribution. Each best fit is obtained with the MATLAB nonlinear least-squares solver {\fontfamily{cmvtt}\selectfont lsqnonlin} \cite{MATLAB:lsqnonlin} with the trust-region-reflective algorithm \cite{Coleman1996}. These data demonstrate that the durations of G1 and S/G2/M, and therefore of the complete cell cycle, are well approximated by a right-truncated Erlang distribution. In Figure~\ref{fig:FigS1}(g) we compare the probability density functions of the exponential and right-truncated Erlang distributions, which clearly demonstrates that these cell cycle durations are not exponentially distributed. Using the {\fontfamily{cmvtt}\selectfont lsqnonlin} solver we find that for each data set the norm of the residual from fitting the right-truncated Erlang distribution is no greater than the norm of the residual from fitting the Erlang distribution. This outcome is expected as the cumulative density of the Erlang distribution tends to one exponentially after the maximum data value. We could also left-truncate the Erlang distribution to ensure a positive lower bound for the distribution, depending on whether a better fit would be achieved with particular data.

\clearpage

\section{Complete proof of Theorem~\ref{main-thrm:NonNeg}}
It suffices to prove that $S(t) \ge 0$ and $F(t) \ge 0$ for all $t > 0$, for then it follows from Lemma~\ref{main-P(t)} that $S(t) \le K$ and $F(t) \le K$ for all $t > 0$. Define $t_1$ and $t_2$ by $t_1 = \inf \{\, t > 0 \mid S(t) < 0 \,\}$ and $t_2 = \inf \{\, t > 0 \mid F(t) < 0 \,\}$. We consider the infima in the extended real numbers, so that $t_1$, $t_2 \in (0,+\infty]$, where either infimum is equal to $+\infty$ if the corresponding set is empty. The proof consists of four separate cases.

\vspace{0.2cm}

Case 1: Let $\beta_S - \beta_F \ge 0$ and suppose $S(t) < 0$ for some $t > 0$.\\
Note that $t_1 \in \RR$. If $t_1 < t_2$ then choose $t_3 \in (t_1,t_2)$ such that $S(t_3) < 0$, $\mathrm{d}S(t) / \mathrm{d}t \, \rvert_{t = t_3} < 0$, and the delays satisfy $\mean{S}(t_3) \ge 0$ and $\mean{F}(t_3) \ge 0$. Then, since $P(t_3) \le K$ by Lemma~\ref{main-P(t)} and since $F(t_3) \ge 0$, Equation~\eqref{main-eq:FS1} gives $\mathrm{d}S(t) / \mathrm{d}t \rvert_{t = t_3} \ge 0$, a contradiction.\\
If $t_1 \ge t_2$ then, since $F(0) > 0$ and $F(t_2) = 0$, there exists $t_3 \in (0,t_2)$ such that $\mathrm{d}F(t) / \mathrm{d}t \rvert_{t = t_3} < 0$. Then, since $P(t_3) \le K$ by Lemma~\ref{main-P(t)}, since the delays satisfy $\mean{S}(t_3) \ge 0$ and $\mean{F}(t_3) \ge 0$, and since $S(t_3)$, $F(t_3) \ge 0$, Equation~\eqref{main-eq:FS2} gives $\mathrm{d}F(t) / \mathrm{d}t \rvert_{t = t_3} \ge 0$, a contradiction. We conclude that $S(t) \ge 0$ for all $t > 0$.

\vspace{0.2cm}

Case 2: Let $\beta_S - \beta_F < 0$ and suppose $S(t) < 0$ for some $t > 0$.\\
Note that $t_1 \in \RR$. If $t_1 \le t_2$ then, since $S(0) > 0$ and $S(t_1) = 0$, there exists $t_3 \in (0,t_1)$ such that $\mathrm{d}S(t) / \mathrm{d}t \rvert_{t = t_3} < 0$. Then, since $P(t_3) \le K$ by Lemma~\ref{main-P(t)}, since the delays satisfy $\mean{S}(t_3) \ge 0$ and $\mean{F}(t_3) \ge 0$, and since $S(t_3)$, $F(t_3) \ge 0$, Equation~\eqref{main-eq:FS1} gives $\mathrm{d}S(t) / \mathrm{d}t \rvert_{t = t_3} \ge 0$, a contradiction.\\
Suppose now that $t_1 > t_2$, and choose $t_3 \in (t_2,t_1)$ such that $F(t_3) < 0$, $\mathrm{d}F(t) / \mathrm{d}t \rvert_{t = t_3} < 0$, and the delays satisfy $\mean{S}(t_3) \ge 0$ and $\mean{F}(t_3) \ge 0$. Then, since $P(t_3) \le K$ by Lemma~\ref{main-P(t)}, and since $S(t_3) \ge 0$, Equation~\eqref{main-eq:FS1} gives $\mathrm{d}F(t) / \mathrm{d}t \rvert_{t = t_3} \ge 0$, a contradiction.\\
Suppose now that $t_1 = t_2$. Since $S(0) > 0$ and $S(t_1) = 0$, there exists $t_3 \in (0,t_1)$ such that $\mathrm{d}S(t) / \mathrm{d}t \rvert_{t = t_3} < 0$. Then, since $P(t_3) \le K$ by Lemma~\ref{main-P(t)}, since the delays satisfy $\mean{S}(t_3) \ge 0$ and $\mean{F}(t_3) \ge 0$, and since $S(t_3)$, $F(t_3) \ge 0$, Equation~\eqref{main-eq:FS2} gives $\mathrm{d}S(t) / \mathrm{d}t \rvert_{t = t_3} \ge 0$, a contradiction. We conclude that $S(t) \ge 0$ for all $t > 0$.

\vspace{0.2cm}

Case 3: Let $\beta_S - \beta_F \ge 0$ and suppose $F(t) < 0$ for some $t > 0$.\\
Note that $t_2 \in \RR$. If $t_2 < t_1$ then, since $F(0) > 0$ and $F(t_2) = 0$, there exists $t_3 \in (0,t_2)$ such that $\mathrm{d}F(t) / \mathrm{d}t \rvert_{t = t_3} < 0$. Then, since $P(t_3) \le K$ by Lemma~\ref{main-P(t)}, since the delays satisfy $\mean{S}(t_3) \ge 0$ and $\mean{F}(t_3) \ge 0$, and since $S(t_3)$, $F(t_3) \ge 0$, Equation~\eqref{main-eq:FS2} gives $\mathrm{d}F(t) / \mathrm{d}t \rvert_{t = t_3} \ge 0$, a contradiction.\\
Suppose now that $t_2 > t_1$, and choose $t_3 \in (t_1,t_2)$ such that $S(t_3) < 0$, $\mathrm{d}S(t) / \mathrm{d}t \rvert_{t = t_3} < 0$, and the delays satisfy $\mean{S}(t_3) \ge 0$ and $\mean{F}(t_3) \ge 0$. Then, since $P(t_3) \le K$ by Lemma~\ref{main-P(t)}, and since $F(t_3) \ge 0$, Equation~\eqref{main-eq:FS1} gives $\mathrm{d}S(t) / \mathrm{d}t \rvert_{t = t_3} \ge 0$, a contradiction.\\
Suppose now that $t_1 = t_2$. Since $F(0) > 0$ and $F(t_2) = 0$, there exists $t_3 \in (0,t_2)$ such that $\mathrm{d}F(t) / \mathrm{d}t \rvert_{t = t_3} < 0$. Then, since $P(t_3) \le K$ by Lemma~\ref{main-P(t)}, since the delays satisfy $\mean{S}(t_3) \ge 0$ and $\mean{F}(t_3) \ge 0$, and since $S(t_3)$, $F(t_3) \ge 0$, Equation~\eqref{main-eq:FS2} gives $\mathrm{d}F(t) / \mathrm{d}t \rvert_{t = t_3} \ge 0$, a contradiction. We conclude that $F(t) \ge 0$ for all $t > 0$.

\vspace{0.2cm}

Case 4: Let $\beta_S - \beta_F < 0$ and suppose $F(t) < 0$ for some $t > 0$.\\
Note that $t_2 \in \RR$. If $t_2 < t_1$ then choose $t_3 \in (t_2,t_1)$ such that $F(t_3) < 0$, $\mathrm{d}F(t) / \mathrm{d}t \rvert_{t = t_3} < 0$, and the delays satisfy $\mean{S}(t_3) \ge 0$ and $\mean{F}(t_3) \ge 0$. Then, since $P(t_3) \le K$ by Lemma~\ref{main-P(t)} and since $S(t_3) \ge 0$, Equation~\eqref{main-eq:FS2} gives $\mathrm{d}F(t) / \mathrm{d}t \rvert_{t = t_3} \ge 0$, a contradiction.\\
Suppose now that $t_2 \ge t_1$. Since $S(0) > 0$ and $S(t_1) = 0$ there exists $t_3 \in (0,t_1)$ such that $\mathrm{d}S(t) / \mathrm{d}t \rvert_{t = t_3} < 0$. Then, since $P(t_3) \le K$ by Lemma~\ref{main-P(t)}, since the delays satisfy $\mean{S}(t_3) \ge 0$ and $\mean{F}(t_3) \ge 0$, and since $S(t_3)$, $F(t_3) \ge 0$, Equation~\eqref{main-eq:FS1} gives $\mathrm{d}S(t) / \mathrm{d}t \rvert_{t = t_3} \ge 0$, a contradiction. We conclude that $F(t) \ge 0$ for all $t > 0$. \qed

\clearpage

\section{Complete proof of Theorem~\ref{main-thrm:Exist}}
We first show that $f$ defined in Equation~\eqref{main-eq:f} satisfies the following Lipschitz condition on every bounded subset of $C$: for all $M > 0$ there exists $L > 0$ such that for $\rho$, $\psi \in C([-\widehat{U},0],\RR^2)$ with $\lVert \rho \rVert$, $\lVert \psi \rVert \le M$ we have $\lVert f(\rho) - f(\psi) \rVert_2 \le L \lVert \rho - \psi \rVert$.

To further simplify the notation in Equation~\eqref{main-eq:f} we define $\kappa_1 = (2\alpha_S - 1) r_S$, $\kappa_2 = 2(1-\alpha_F) r_F$, $\kappa_3 = 2(1-\alpha_S) r_S$, $\kappa_4 = (2\alpha_F - 1) r_F$, and $\kappa_5 = (\beta_S - \beta_F) / K$. Now,
\begingroup
\allowdisplaybreaks
\begin{align*}
f(\rho) - f(\psi) &=
\left[
\begin{array}{ll}
\displaystyle \Big(\kappa_1 \mean{\rho_S} + \kappa_2 \mean{\rho_F} \Big) \bigg(1 - \frac{(\rho_S + \rho_F) (0)}{K}\bigg)
- \kappa_5 \rho_S (0) \rho_F (0) \\[0.5cm]
\displaystyle - \Big(\kappa_1 \mean{\psi_S} + \kappa_2 \mean{\psi_F} \Big) \bigg(1 - \frac{(\psi_S + \psi_F) (0)}{K}\bigg)
+ \kappa_5 \psi_S (0) \psi_F (0) \\[1cm]
\displaystyle \Big(\kappa_3 \mean{\rho_S} + \kappa_4 \mean{\rho_F} \Big) \bigg(1 - \frac{(\rho_S + \rho_F) (0)}{K}\bigg)
+ \kappa_5 \rho_S (0) \rho_F (0) \\[0.5cm]
\displaystyle - \Big(\kappa_3 \mean{\psi_S} + \kappa_4 \mean{\psi_F} \Big) \bigg(1 - \frac{(\psi_S + \psi_F) (0)}{K}\bigg)
- \kappa_5 \psi_S (0) \psi_F (0) \\
\end{array}
\right] \\[0.5cm]
&=
\left[
\begin{array}{ll}
\displaystyle \big(\kappa_1 ( \mean{\rho_S} - \mean{\psi_S} ) + \kappa_2 ( \mean{\rho_F} - \mean{\psi_F} ) \big) \bigg(1 - \frac{(\rho_S + \rho_F) (0)}{K}\bigg) \\[0.5cm]
\displaystyle + \Big(\kappa_1 \mean{\psi_S} + \kappa_2 \mean{\psi_F} \Big) \bigg(\frac{(\psi_S - \rho_S) (0) + (\psi_F - \rho_F) (0)}{K}\bigg) \\[0.5cm]
+ \kappa_5 (\psi_S - \rho_S) (0) \psi_F (0) + \kappa_5 (\psi_F - \rho_F) (0) \rho_S (0) \\[1cm]
\displaystyle \big(\kappa_3 ( \mean{\rho_S} - \mean{\psi_S} ) + \kappa_4 ( \mean{\rho_F} - \mean{\psi_F} ) \big) \bigg(1 - \frac{(\rho_S + \rho_F) (0)}{K}\bigg) \\[0.5cm]
\displaystyle + \Big(\kappa_3 \mean{\psi_S} + \kappa_4 \mean{\psi_F} \Big) \bigg(\frac{(\psi_S - \rho_S) (0) + (\psi_F - \rho_F) (0)}{K}\bigg) \\[0.5cm]
+ \kappa_5 (\rho_S - \psi_S)(0) \psi_F (0) + \kappa_5 ( \rho_F - \psi_F)(0) \rho_S (0)
\end{array}
\right]
\end{align*}
\endgroup
so, using the triangle inequality, we obtain
\begingroup
\allowdisplaybreaks
\begin{align*}
\lVert f(\rho) - f(\psi) \rVert_2 &\le
\left\lVert \left[
\begin{array}{ll}
\displaystyle \kappa_1 ( \mean{\rho_S} - \mean{\psi_S} ) \bigg(1 - \frac{(\rho_S + \rho_F) (0)}{K}\bigg) \\[0.7cm]
\displaystyle \kappa_3 ( \mean{\rho_S} - \mean{\psi_S} ) \bigg(1 - \frac{(\rho_S + \rho_F) (0)}{K}\bigg)
\end{array}
\right] \right\rVert_2 \\[0.5cm]
&\quad + \left\lVert \left[
\begin{array}{ll}
\displaystyle \kappa_2 ( \mean{\rho_F} - \mean{\psi_F} ) \bigg(1 - \frac{(\rho_S + \rho_F) (0)}{K}\bigg) \\[0.7cm]
\displaystyle \kappa_4 ( \mean{\rho_F} - \mean{\psi_F} ) \bigg(1 - \frac{(\rho_S + \rho_F) (0)}{K}\bigg)
\end{array}
\right] \right\rVert_2 \\[0.5cm]
&\quad +
\left\lVert \left[
\begin{array}{ll}
\displaystyle \kappa_1 \mean{\psi_S} \bigg(\frac{(\psi_S - \rho_S) (0) + (\psi_F - \rho_F) (0)}{K}\bigg) \\[0.7cm]
\displaystyle \kappa_3 \mean{\psi_S} \bigg(\frac{(\psi_S - \rho_S) (0) + (\psi_F - \rho_F) (0)}{K}\bigg) \\
\end{array}
\right] \right\rVert_2 \\[0.5cm]
&\quad + \left\lVert \left[
\begin{array}{ll}
\displaystyle \kappa_2 \mean{\psi_F} \bigg(\frac{(\psi_S - \rho_S) (0) + (\psi_F - \rho_F) (0)}{K}\bigg) \\[0.7cm]
\displaystyle \kappa_4 \mean{\psi_F} \bigg(\frac{(\psi_S - \rho_S) (0) + (\psi_F - \rho_F) (0)}{K}\bigg) \\
\end{array}
\right] \right\rVert_2 \\[0.5cm]
&\quad +
\left\lVert \left[
\begin{array}{ll}
\kappa_5 (\psi_S - \rho_S) (0) \psi_F (0) \\[0.5cm]
\kappa_5 (\rho_S - \psi_S) (0) \psi_F (0) \\
\end{array}
\right] \right\rVert_2 + 
\left\lVert \left[
\begin{array}{ll}
\kappa_5 (\psi_F - \rho_F) (0) \rho_S (0) \\[0.5cm]
\kappa_5 ( \rho_F - \psi_F)(0) \rho_S (0)\\
\end{array}
\right] \right\rVert_2 \\[0.5cm]
&\le \sqrt{\kappa_1^2 + \kappa_3^2} \Big(1 + \frac{1}{K} \lvert \rho_S (0) \rvert + \frac{1}{K} \lvert \rho_F (0) \rvert \Big) \lvert ( \mean{\rho_S} - \mean{\psi_S} ) \rvert \\[0.5cm]
&\quad + 
\sqrt{\kappa_2^2 + \kappa_4^2} \Big(1 + \frac{1}{K} \lvert \rho_S (0) \rvert + \frac{1}{K} \lvert \rho_F (0) \rvert \Big) \lvert ( \mean{\rho_F} - \mean{\psi_F} ) \rvert \\[0.5cm]
&\quad +
\frac{1}{K} \sqrt{\kappa_1^2 + \kappa_3^2} \lvert \mean{\psi_S} \rvert \lvert (\psi_S - \rho_S) (0) + (\psi_F - \rho_F) (0) \rvert \\[0.5cm]
&\quad +
\frac{1}{K} \sqrt{\kappa_2^2 + \kappa_4^2} \lvert \mean{\psi_F} \rvert \lvert (\psi_S - \rho_S) (0) + (\psi_F - \rho_F) (0) \rvert \\[0.5cm]
&\quad + \sqrt{2} \left| \kappa_5 \right| \left| (\rho_S - \psi_S) (0) \right| \left| \psi_F (0) \right| + \sqrt{2} \left| \kappa_5 \right| \left| (\rho_F - \psi_F) (0) \right| \left| \rho_S (0) \right| \\[0.5cm]
&\le \sqrt{\kappa_1^2 + \kappa_3^2} \Big(1 + \frac{1}{K} \lVert \rho_S \rVert + \frac{1}{K} \lVert \rho_F \rVert \Big) \lVert \rho_S - \psi_S \rVert \\[0.5cm]
&\quad + 
\sqrt{\kappa_2^2 + \kappa_4^2} \Big(1 + \frac{1}{K} \lVert \rho_S \rVert + \frac{1}{K} \lVert \rho_F \rVert \Big) \lVert \rho_F - \psi_F \rVert \\[0.5cm]
&\quad +
\frac{1}{K} \sqrt{\kappa_1^2 + \kappa_3^2} \lVert \psi_S \rVert \big( \lVert \psi_S - \rho_S \rVert + \lVert \psi_F - \rho_F \rVert \big) \\[0.5cm]
&\quad +
\frac{1}{K} \sqrt{\kappa_2^2 + \kappa_4^2} \lVert \psi_F \rVert \big( \lVert \psi_S - \rho_S \rVert + \lVert \psi_F - \rho_F \rVert \big) \\[0.5cm]
&\quad + \sqrt{2} \lvert \kappa_5 \rvert \lVert \rho_S - \psi_S \rVert \lVert \psi_F \rVert + \sqrt{2} \lvert \kappa_5 \rvert \lVert \rho_F - \psi_F \rVert \lVert \rho_S \rVert \\[0.5cm]
&\le \bigg(\sqrt{\kappa_1^2 + \kappa_3^2} \Big(1 + \frac{2M}{K} \Big) 
+ \sqrt{\kappa_2^2 + \kappa_4^2} \Big(1 + \frac{2M}{K} \Big) 
+ \frac{2M}{K} \sqrt{\kappa_1^2 + \kappa_3^2} \\[0.5cm]
& \qquad + \frac{2M}{K} \sqrt{\kappa_2^2 + \kappa_4^2} 
+ 2 \sqrt{2} \lvert \kappa_5 \rvert M \bigg) \lVert \rho - \psi \rVert \\[0.5cm]
&= \Bigg(\bigg(\sqrt{\kappa_1^2 + \kappa_3^2} + \sqrt{\kappa_2^2 + \kappa_4^2}\bigg) \bigg(1 + \frac{4M}{K} \bigg) 
+ 2 \sqrt{2} \lvert \kappa_5 \rvert M \Bigg) \lVert \rho - \psi \rVert,
\end{align*}
so we can set $L$ to be
\begin{equation*}
L = \bigg(\sqrt{\kappa_1^2 + \kappa_3^2} + \sqrt{\kappa_2^2 + \kappa_4^2}\bigg) \bigg(1 + \frac{4M}{K} \bigg) 
+ 2 \sqrt{2} \lvert \kappa_5 \rvert M
\end{equation*}
\endgroup
and then $f$ satisfies the Lipschitz condition. Then \cite[Page 32, Theorem 3.7]{Smith2011} provides local existence and uniqueness of solutions for the system \eqref{main-eq:FS1} and \eqref{main-eq:FS2}. Since our solutions of interest are bounded by Theorem~\ref{main-thrm:NonNeg}, it follows from \cite[Page 37, Proposition 3.10]{Smith2011} that the solutions are continuable to all positive time. \qed

\clearpage

\section{Alternative proof of Proposition~\ref{main-prop:Equil0}}
The functions $S$ and $F$ are non-negative by Theorem~\ref{main-thrm:NonNeg}, so the following inequalities show that the equilibrium point $(S^{\text{*}},F^{\text{*}}) = (0,0) \in C([-\widehat{U},\infty),\RR_{\ge 0}^2)$ for the system \eqref{main-eq:FS1} and \eqref{main-eq:FS2} is stable if and only if the equilibrium point $P^{\text{*}} = 0 \in C([-\widehat{U},\infty),\RR_{\ge 0})$ for Equation~\eqref{main-eq:Sum} is stable:
\begin{equation}\label{eq:Ineq}
\lVert (S,F) \rVert \le \lVert P \rVert \le \sqrt{2} \, \lVert (S,F) \rVert.
\end{equation}
The history function $\phi$ for the system \eqref{main-eq:FS1} and \eqref{main-eq:FS2} is strictly positive by Equation~\eqref{main-eq:history1}, and $\phi_S + \phi_F < K$ by Equation~\eqref{main-eq:history2}. It follows by continuity that $S(t) > 0$, $F(t) > 0$, and $S(t) + F(t) < K$ in a neighbourhood of $(0,0)$. So, by Equation~\eqref{main-eq:Sum}, $\mathrm{d}P(t) / \mathrm{d}t > 0$ in a neighbourhood of $P^{\text{*}} = 0$, which is therefore an unstable equilibrium point. We conclude that $(S^{\text{*}},F^{\text{*}}) = (0,0)$ is also an unstable equilibrium point by Equation~\eqref{eq:Ineq}. \qed

\clearpage

\section{Graphical illustration of Cauchy's argument principle}
In Figure~\ref{fig:FigS2} we graphically illustrate our application of Cauchy's argument principle.
\begin{figure}[p]
\includegraphics[width=0.7\textwidth]{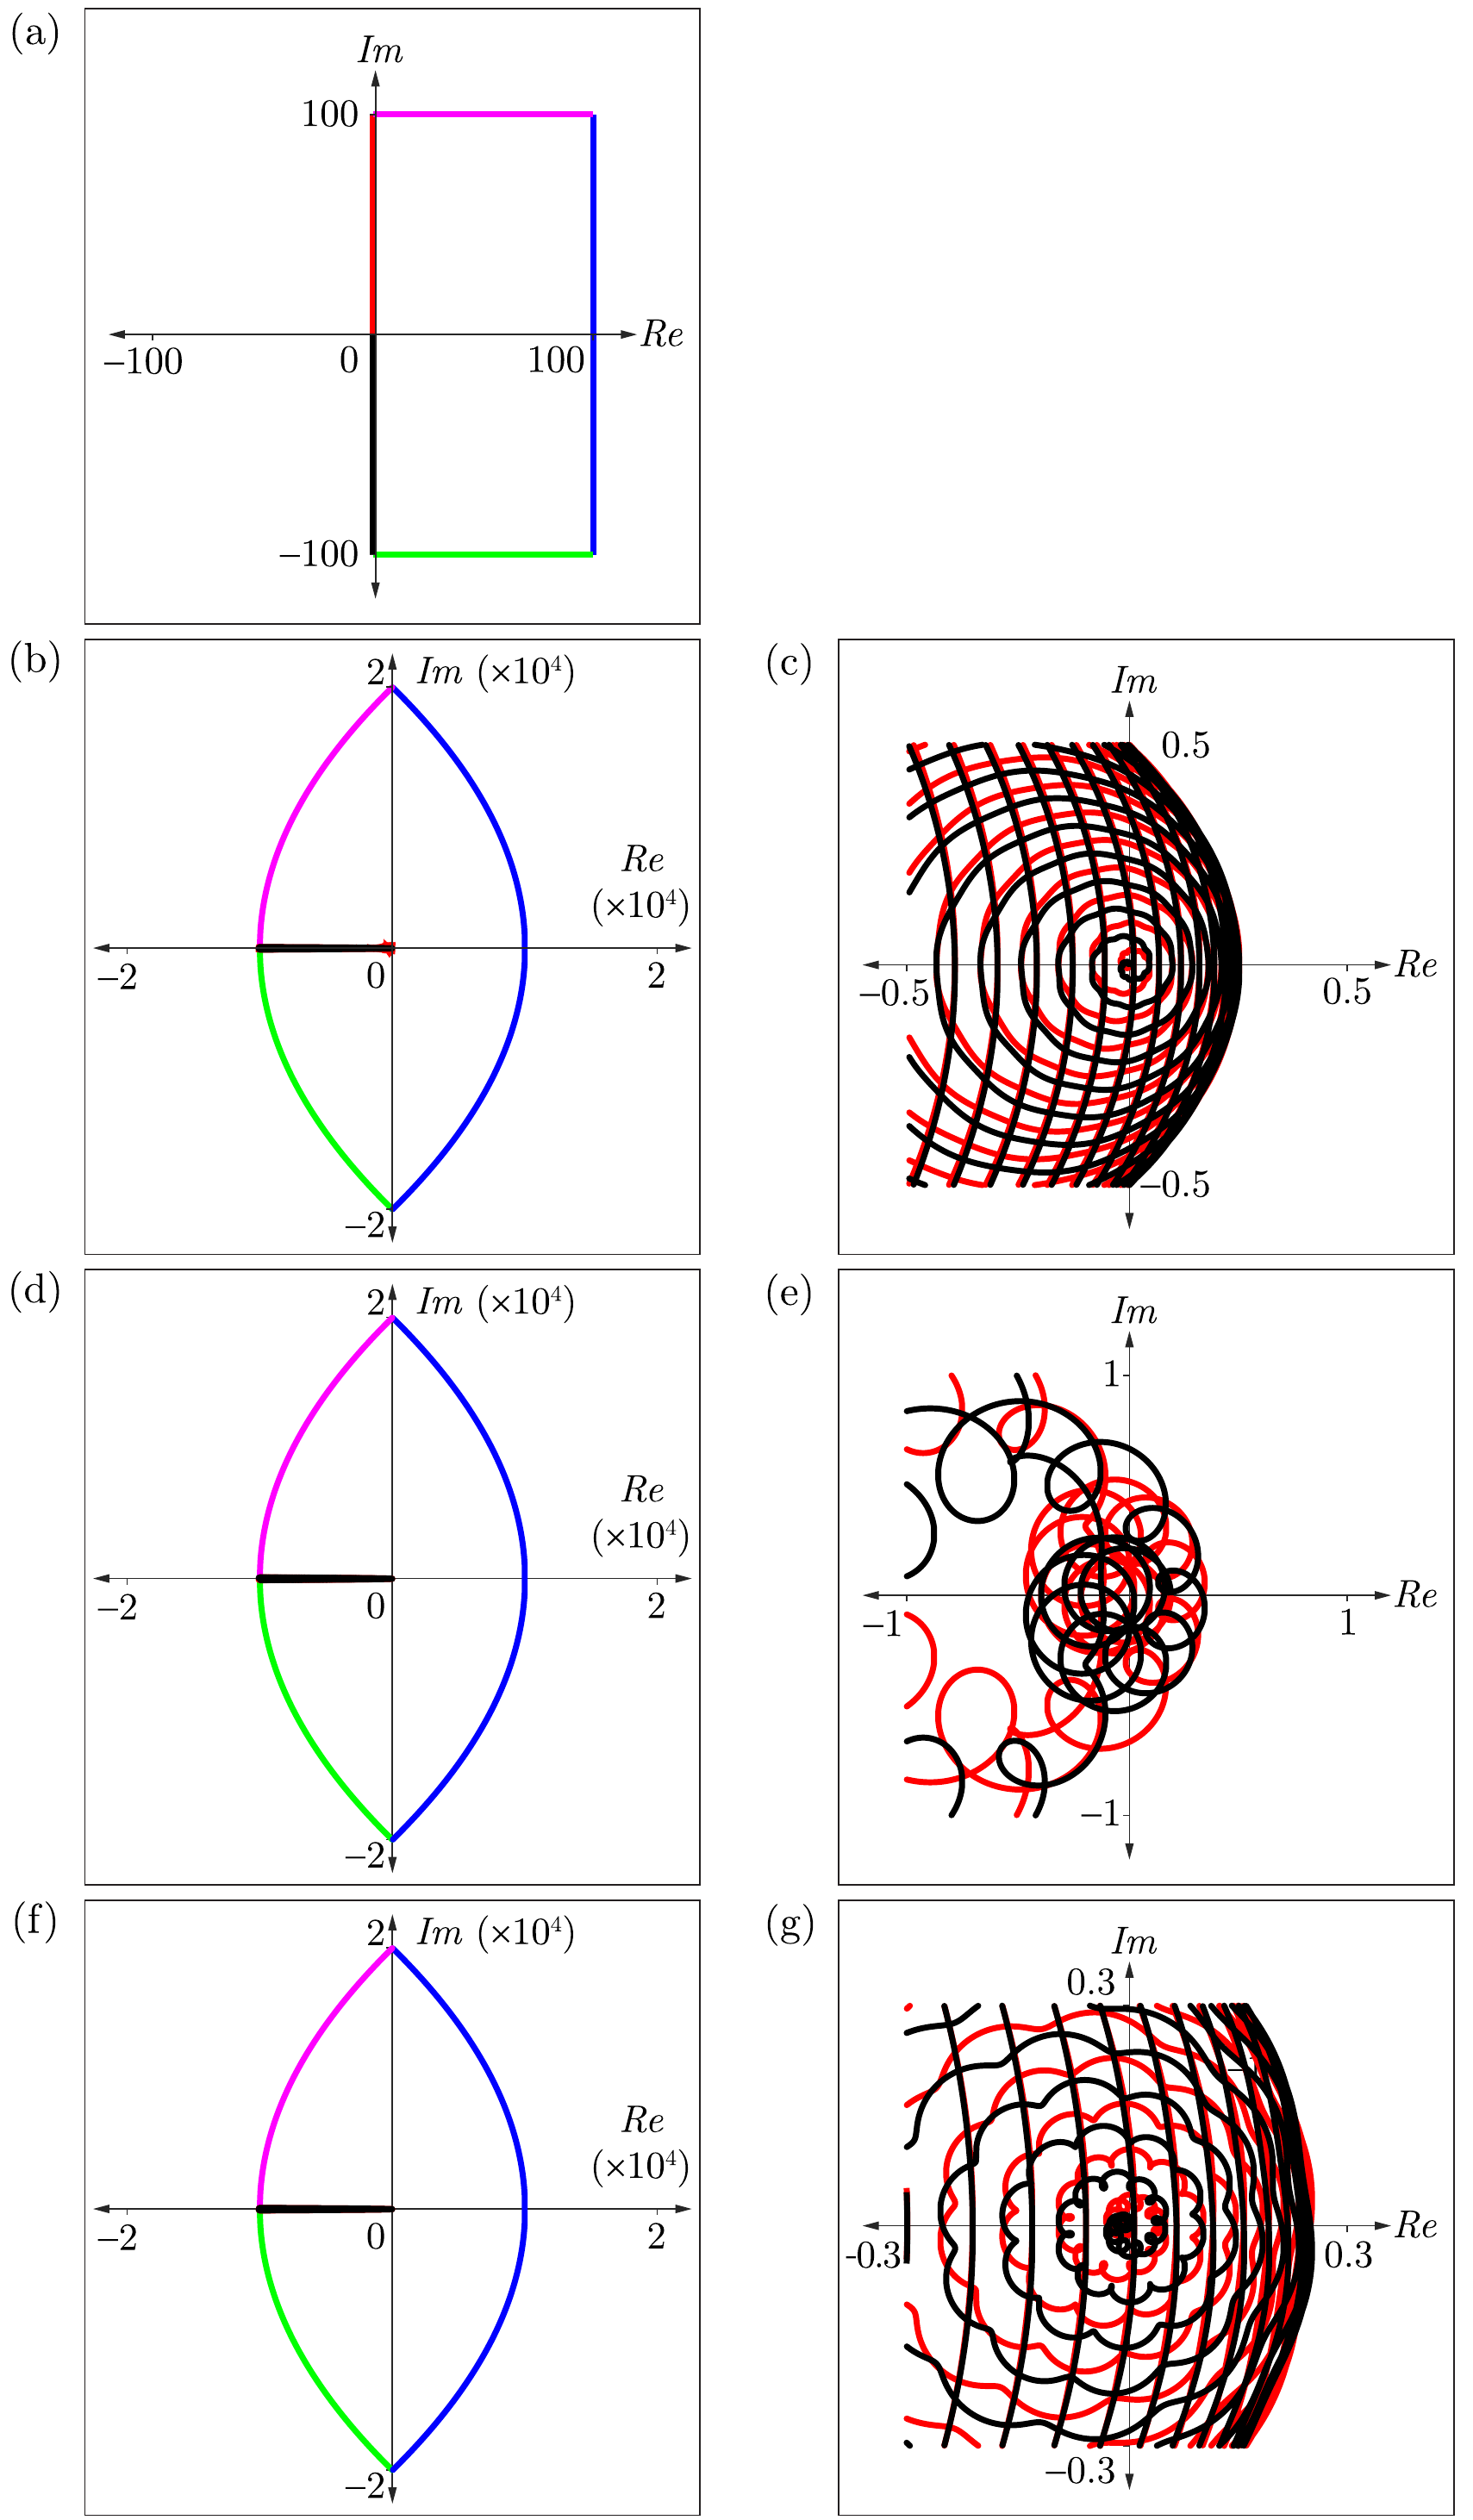}
\caption{Graphical illustration of our application of Cauchy's argument principle for $G_{\delta}(\lambda)$ in Equation~\eqref{eq:Transcendental_discrete}, when $2 \alpha_S + 2 \alpha_F - 3 > 0$. (a) A rectangular contour $\Gamma$ in the right half-plane does not intersect the imaginary axis. (b) The image contour $G_{\delta}(\Gamma)$ when $G_{\delta}$ has the parameters $\alpha_S = 0.6$, $\alpha_F = 1$, $r_F = 1$, and $r = 0.01$, with a close-up view of the origin in (c). (d) The image contour $G_{\delta}(\gamma)$ when $G_{\delta}$ has the parameters $\alpha_S = 0.6$, $\alpha_F = 1$, $r_F = 0.1$, and $r = 1$, with a close-up view of the origin in (e). (f) The image contour $G_{\delta}(\Gamma)$ when $G_{\delta}$ has the parameters $\alpha_S = 1$, $\alpha_F = 1$, $r_F = 1$, and $r = 0.01$, with a close-up view of the origin in (g). Each coloured segment of $G_{\delta}(\Gamma)$ in (b)--(f) is the image of the same-coloured segment of the rectangular contour $\Gamma$ in (a) under $G_{\delta}(\lambda)$}
\label{fig:FigS2}
\end{figure}
We let $\Gamma$ be the closed rectangular contour in Figure~\ref{fig:FigS2}(a). Due to the integrals in the transcendental characteristic equation $G(\lambda)$ in Equation~\eqref{main-eq:Transcendental}, a very large number of numerical integrations are required to calculate $G(\lambda)$ along a contour. So, we instead use the discrete delay version of $G(\lambda)$, denoted by $G_{\delta}(\lambda)$, which gives similar qualitative behaviour:
\begin{equation}
G_{\delta}(\lambda) = \lambda^2 - \lambda \Big((2\alpha_S - 1) r e^{-\lambda r_F \tau_S}  + (2\alpha_F - 1) e^{-\lambda r_F \tau_F} \Big) + (2\alpha_S + 2\alpha_F - 3) r e^{-\lambda r_F (\tau_S + \tau_F)}\, , \label{eq:Transcendental_discrete}
\end{equation}
obtained from $G(\lambda)$ with the Dirac kernels $g_S (z) = \delta (z-\tau_S)$ and $g_F (z) = \delta (z-\tau_F)$ for discrete delays $\tau_S$ and $\tau_F$. Figures~\ref{fig:FigS2}(b), (d), and (f) show the images $G_{\delta}(\Gamma)$ for three different sets of parameters for $G_{\delta}(\lambda)$, and Figures~\ref{fig:FigS2}(c), (e), and (g) show the respective close-up views around the origin. Note that each coloured segment of $G_{\delta}(\Gamma)$ in (b)--(f) is the image of the same-coloured segment of the rectangular contour $\Gamma$ in (a) under $G_{\delta}(\lambda)$. To calculate the winding number of $G_{\delta}(\Gamma)$ with respect to the origin we count the net number of times that $G_{\delta}(\Gamma)$ winds counter-clockwise around the origin, assigning $+1$ for each time $G_{\delta}(\Gamma)$ winds around the origin in a counter-clockwise direction, and $-1$ for each time $G_{\delta}(\Gamma)$ winds around the origin in a clockwise direction. Figure~\ref{fig:FigS2} illustrates that the behaviour of $G_{\delta}(\Gamma)$ can be complicated near the origin, so when calculating the winding number of $G_{\delta}(\Gamma)$ with respect to the origin we need to ensure that we also account for the possibility of $G_{\delta}(\Gamma)$ winding around the origin in a clockwise direction.

\clearpage

\addcontentsline{toc}{section}{References}

\newpage

\bibliography{SeanBibliography}
\bibliographystyle{vancouver}

\end{document}
